# Supplementary material for: Efficient Convex Optimization Requires Superlinear Memory
Source: arXiv:2203.15260 source file (2024-07-24)
Supplement: Supplementary file 2 [file generalgapresults.tex]

\subsection{Results for general convergence rates}
\label{appendix:generalgapbounds}
Suppose we re-defined the fourth criterion of a {\functionclassname}   to be that for any (potentially randomized) algorithm $\algrand$, if $r \leq \nnem$ then for any $i \leq t_r$, 
\begin{equation}
    F_{f, \A}(\x_i) - F_{f, \A}(\x \opt) \geq g(\nnem),
\end{equation}
where $g(\nnem)$ is some non-increasing, invertible function. We call $\functionclass$ a $(L, \nnem, g)$-{\functionclassname} in this case. Then we have the following theorem. 
\begin{theorem}
Let $\left \{ B_d \right \}_{d = 1}^{\infty}$ be a memory-sensitive base and $\mathcal{F}$ be an $(L, \nnem, g)$-\functionclassname. Suppose $\A = \left( \vec{a}_1, \dots, \vec{a}_n \right)^{\top}$ for $\vec{a}_i \simiid \mathsf{Unif}(B_d)$ and $f \sim \functionclass$. For $\epsilon = g(\nnem)$, any algorithm constrained to working with memory with size at most $\memsize$ which outputs an $\epsilon$-optimal point for $F_{f, \A}$ with failure probability at most $\failureprobalg$ requires at least 
\begin{equation}
    \frac{c g^{-1}(\epsilon) d^2 (1 - \failureprob - \failureprobalg)}{\memsize},
\end{equation}
many first-order oracle queries, where $c > 0$ is an absolute constant (independent of $d$). 
\end{theorem}
